# Supplementary material for: Visualizing Information on Smartwatch Faces: A Review and Design Space
Source: arXiv:2310.16185 source file (2024-01-12)
Supplement: Supplementary file 1 [file 09-appendix_old.tex]

% \section*{Appendix}
\begin{table*}
	 \caption{Four examples of smartwatch faces describing design space dimensions.}
	
\centering 
    \begin{tabular}{ m{1cm} m{5cm} m{10cm} }
    \toprule
	& Smartwatch face & Design space dimensions  \\
	\midrule
 a) & \includegraphics[width=.5\columnwidth]{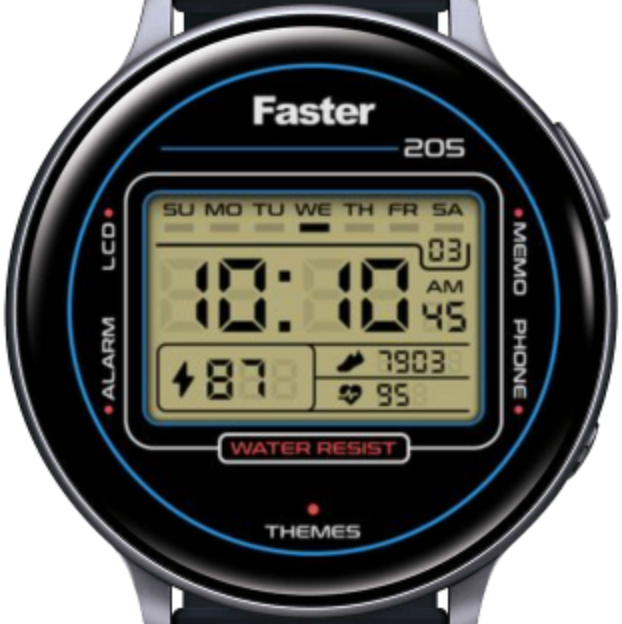} & \textbf{Factors}: This watch face (designed by--Faster Studio, Facer) was designed for full color round watch displays. It is meant to show relatively basic smart watch data and to serve primarily as a time piece.  \textbf{Style/Theme}: This watch face  imitates but updates some of the oldest retro digital watches which is visible through the choice of the overall color scheme that matches old digital watches and the semi-flat design. \textbf{Components}: The watch face chose only three complications: battery life, step count, and heart rate next to the time and date display. Graphical decorators are used to give the impression of an old digital watch. \textbf{Representations:} The overall theme of the watch has a direct influence on the size and representations of components. A large amount of space is dedicated to decorators that give the graphical context of digital watches. The largest components in the square central container show time and date. The more modern smart watch functions are displayed as text with small icons as labels using old digital watch fonts.\\
 \\
 
  b) & \includegraphics[width=.5\columnwidth]{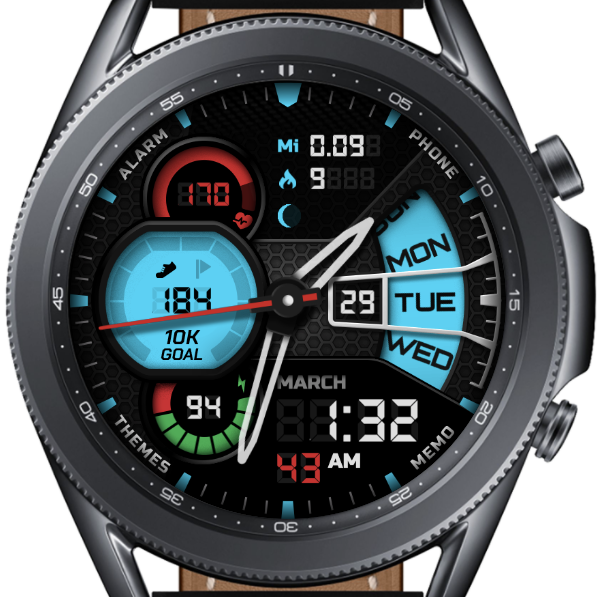} & \textbf{Factors:} This watch face (designed by--BERGEN, Facer) compactly assembles necessary health information that quickly grabs health \& fitness-conscious people's attention. This design is meant to fit in both square, and round shape watch faces. \textbf{Style/Theme:} This watch face has a modern, stylish look with a vibrant presentation on a skeuomorphism interface. It used three hues on a black theme color palette, including red, neon blue, and green. The neon blue color does not only reflect the trend but also gives a luxurious touch to the watch face. \textbf{Components:} Six complications, i.\,e., heart rate, step count, battery charge, distance traveled, calories burned, moon phase, including timestamp, make this watch face informative but at the same time displays a lot of data to the wearers. \textbf{Representations:} It is interesting to observe some visualization complications; for example, heart rate and step count represent data with the combination of Icon+Text+Chart.\\
  
    c) & \includegraphics[width=.5\columnwidth]{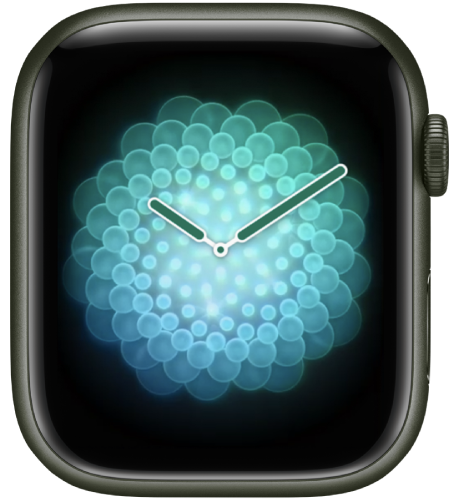} &
    \bigskip
    \textbf{Factors:} This watch face (designed by--Apple~\cite{Apple-Watch-Face:2022}) is aimed at helping wearers relax in sync with soothing animation. \textbf{Style/Theme:} The patterns in the animated image with the calming color palette are meant to create a soothing feel. Wearers inhale while the animation grows and exhales as the animation shrinks. \textbf{Components:} The watch face only shows time data as an analog watch representation on a semi-flat interface. \textbf{Representations:} This watch face has no other complications except time and only uses an animated background image.\\
  
   d) & \includegraphics[width=.5\columnwidth]{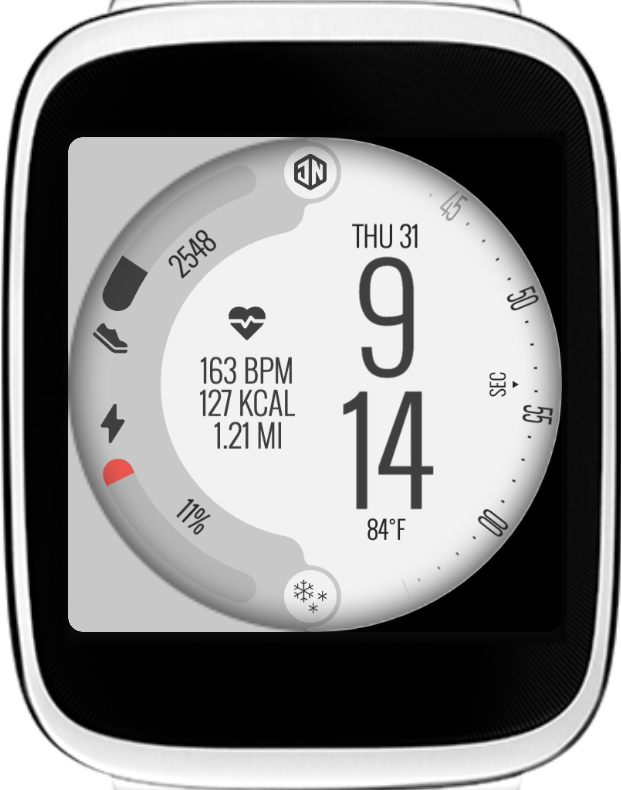} & 
\textbf{Factors:} This watch face (designed by– JN WatchFaces, Facer) was designed for both round and square type watch displays. The left side arc disappears when it displays on a round-shaped watch face. \textbf{Style/Theme:} The unique second dial makes this watch face different; while its minimalistic color palette creates an aesthetically pleasing result. The sparing use of vibrant red color in one complication enforces the minimalistic design. \textbf{Components:} It shows heart rate, step count, temperature, sky condition, calories burned, distance traveled, and battery charging complications, including a timestamp. \textbf{Representations:} Two complications, step count and watch battery charging, are represented with chart+icon+text, where the Icon is used as a label. For others, sky condition is represented with Icon only, heart rate with Icon+Text and other complications are represented with simple text.\\
	\midrule
	    \bottomrule
  \end{tabular}
 \label{tab:design_space_examplary_watch_faces}
\end{table*}
